# Supplementary material for: Combinatorial Multi-Armed Bandit and Its Extension to Probabilistically Triggered Arms
Source: arXiv:1407.8339 source file (2016-03-29)
Supplement: Supplementary file 1 [file appendix.tex]

\clearpage

\onecolumn

\appendix

\setcounter{equation}{13}
\setcounter{mythm}{2}
\section*{Supplementary Material}

\begin{mylem}[Bernstein inequality]\label{bernstein}
Let $\myX_1,\dots, \myX_\myn$ be independent zero-mean random variables. If
for all $1\leq\myi\leq\myn, |\myX_\myi|\leq \myM$, then for all $\myt>0$,
\[\Pr \left[\left|\sum_{\myi=1}^\myn \myX_\myi\right|>\myt\right] \leq \exp\left\{-\frac{\myt^2/2}
{\sum_{\myi=1}^\myn \mathbb{E} [\myX_\myi^2]+\myM\myt/3}\right\}.\]
\end{mylem}

\section{CMAB with Clustered Arms}

\label{sec:clusteredbandit}

In many applications, multiple arms are clustered and are always played together.
For example, in the PMC bandit problem, all arms (edges) incident to a node in $L$ are
	always played together; in the influence maximization bandit problem, all arms (outgoing
	edges) from the same node are always played together.
In this section, we show how to take advantage of such arm clusters to further
	improve the regret analysis.

We consider the following CMAB problem with clustered arms. Formally, each cluster $C \subseteq [m]$ contains a set of simple arms.
Denote $\newU$ as the set of all clusters. Notice that one arm may belong to multiple clusters.
We assume $|\newU| < m$. In this setting, each super arm $S$ is a union of several clusters: $S=\bigcup_{C\in g(S)} C$, where
	$g(S)$ is the set of clusters that forms $S$.
When super arm $S$ is played in round $t$, the outcomes of all arms in the clusters in $S$ will be revealed.

We will use the same CUCB algorithm with a minor change to the initialization rounds: In the first $|U|$ rounds of initialization, for each cluster $C$, we play a super arm $S$ such that $C\in g(S)$ and update variables $\hat{\mu}_i$ accordingly.

For a given cluster $C\subseteq [m]$, we sort all {\em bad} super arms whose
cluster set
contains $C$
as $S_{C,B}^1, S_{C,B}^2, \cdots, S_{C,B}^{K_C}$ by
increasing reward. Define
\begin{equation}
\label{eqn:deltaij:cluster}
\Delta^{C,j} = \alpha \cdot \opt_{\bp} - r_{\bp}(S_{C,\bad}^j),
\end{equation}
$\Delta_{\max}^C = \Delta^{C,1}$ and  $\Delta_{\min}^C = \Delta^{C, K_C}$.
If $C$ does not belong to any {\em bad} super arm, $K_C = 0$ and set $\Delta_{\max}^C = \Delta_{\min}^C = 0$.
Furthermore, define $\Delta_{\max}=\max_{C\in U} \Delta_{\max}^C$.

\def\thmclustered{
Consider the CMAB problem with the set of clusters $U$ of arms.
In $n$ rounds
	the $(\alpha,\beta)$-approximation regret of the CUCB algorithm
	using an $(\alpha,\beta)$-approximation
	oracle is at most
\[
\sum_{C\,\mid\, \Delta_{\min}^C > 0}\left(
\frac{6\ln n}{(f^{-1}(\Delta^C_{\min}))^2}\cdot \Delta^C_{\min}
%\ell_n(\Delta^{C,K_C}) \Delta^{C,K_C}
+ \int_{\Delta^{C}_{\min}}^{\Delta^{C}_{\max}} \frac{6\ln n}{(f^{-1}(x))^2} \mathrm{d}x\right)
+ \left(\frac{\pi^2}{3}+1\right)\cdot m \cdot \Delta_{\max}.
\]
}

\begin{mythm} \label{thm:clustered}
{\thmclustered}
\end{mythm}
\paragraph{Discussion.} Comparing with the
regret bound in Theorem~1, we are taking the summation over all clusters instead of all underlying arms. Since we assume $|U|<m$, intuitively, we could be better off. However, it is not clear how the $\Delta_{\min}$'s of the underlying arms and clusters are correlated with each other.
When clusters do not intersect with one another and thus form a partition of the underlying
	arms, it is straightforward to show that $\Delta_{\min}^i = \Delta_{\min}^C$ if
	the cluster $C$ contains the arm $i$.
In this case, the new regret bound of Theorem~\ref{thm:clustered} is a strict
	improvement over Theorem~1.
The two applications discussed in this paper, i.e., the bandit PMC problem and the bandit influence maximization problem, belong to this category and thus Theorem~\ref{thm:clustered}
could be applied and obtain improved regret bounds.

\begin{proof}
The proof of this theorem is almost identical 
to Theorem~1. In addition to $T_i$, our analysis requires $T_\newu$ which is the number of
time cluster $C$ is selected to play.
Let $T_{\newu,n}$ be the value of $T_\newu$ at the end of round $n$,
	that is, $T_{\newu,n}$ is the number of times cluster $\newu$ is played in the
	first $n$ rounds.
Let $T_{i,n}$ still be the value of $T_i$ at the end of round $n$,
	that is, $T_{i,n}$ is the number of times arm $i$ is played in the
	first $n$ rounds.
Since arm $i$ might be contained in multiple clusters, here $T_{i,n}$
    is larger than $T_{\newu,n}$ for any $\newu$ containing $i$.

For the proof, we maintain counter $N_\newu$ for each cluster
$\newu$ after
	the $\newU$ initialization rounds.
Let $N_{\newu,t}$
  be the value of $N_\newu$ after the $t$-th round and $N_{\newu,|\newU|} = 1$.
Note that  $\sum_{\newu}N_{\newu,|\newU|}=|\newU|$.
  $\{N_\newu\}$ is updated in the following way.

For a round $t>|U|$, let $S_t$ be the super arm selected in round $t$.
Round $t$ is bad if the oracle selects a super arm $S_t\in \calS_\bad$,
which is not an $\alpha$-approximate super arm. If round $t$ is bad,
let $\newu =
  \argmin_{\newu\in g(S_t)} N_{\newu,t-1} $ and increment $N_{\newu}$ by one,
  i.e., $N_{\newu,t} = N_{\newu,t-1}+1$. In other words, we find
  the cluster $C$ with smallest counter in $g(S_t)$ and increase its counter.
   If $\newu$ is not
  unique, we pick an arbitrary cluster with the smallest counter in
  $g(S_t)$.

By definition $N_{\newu,t} \leq T_{\newu,t}$.
The total number of bad rounds in the first
$n$ rounds is $\sum_{\newu}N_{\newu,n}$.
%We then investigate
%$\sum_{\newu}N_{\newu,n}$
%from the perspective of
%super arms.

Each time $N_C$ gets updated, one of the bad arm whose cluster set
contains $C$ is played. We further divide $N_C$ into more counters as follows:

\[\forall l\in [K_C],\, N_{C,n}^l = \sum_{t=|U|+1}^n \I\{S_t = S_{C,\bad}^l, N_{C,t}>N_{C,t-1}\}.\]

%Define $\base_t = \frac{
% 4\ln t +2\ln\ln t
% }{\left(f^{-1}\left({\Delta_{\min}}\right)\right)^2}$.
%Consider a BAD round $t$, $S_t\in \calS_\bad$ is selected
%and counter $N_\newu$ is
% updated.  There are two possible cases: (1) $N_{\newu,t-1}\leq \base_t$; (2)
% $N_{\newu,t-1}> \base_t$.
%We define the second event as $\rare_{t}$, i.e.,
%a counter greater than $\base_t$ gets updated in a BAD round $t$.

Define $\base_n(\Delta)=\frac{6\ln n }{(f^{-1}(\Delta))^2}$.
When counter $N_{i,t}^l$ is increased at time $t$,
i.e., $S_t=S_{C,B}^l$, we inspect the counter $N_{C,t-1}^l$.
Notice that $N_{C,t-1}^l$ is
the smallest time that all arms in $S_t$ have been
played.
If $N_{c,t-1}>\base_n (\Delta^{C,l})$, we call the bad arm
$S_{C,B}^l$ is sufficiently sampled. Otherwise,
it is under-sampled. We write as
\begin{align*}
N_{C,n}^{l, suf} =& \sum_{t=m+1}^n \I\{S_t = S_{C,\bad}^l, N_{C,t}>N_{C,t-1}, N_{C,t-1} > \ell_n(\Delta^{C,l})\}, \nonumber \\
N_{C,n}^{l, und} =& \sum_{t=m+1}^n \I\{S_t = S_{C,\bad}^l, N_{C,t}>N_{C,t-1}, N_{C,t-1} \le \ell_n(\Delta^{C,l})\}.
\end{align*}

Then we have $N_{C,n} = 1+\sum_{l\in [K_C]} (N_{C,n}^{l, suf} + N_{C,n}^{l, und})$. Using this notation, the total reward at time horizon $n$ is at least

\begin{equation}
\label{eqn:reward:cluster}
n\cdot \alpha \cdot \opt_{\bp} - \sum_{C\in U}\left(\Delta^{C,1} + \sum_{l\in [K_C]} (N_{C,n}^{l, suf} + N_{C,n}^{l, und}) \cdot \Delta^{C,l}\right).
\end{equation}

Note that the total sampled time of
underlying arms in one cluster will not be smaller than
the total sampled time of
that cluster.
We claim that it is unlikely that a bad super arm is played when all the underlying arms are sufficiently sampled.
In other words, for a bad super arm, if all its underlying arms are sufficiently sampled, it should not be played in the first place. More specifically, we have the following claim.

\begin{mylem} For any time horizon $n > m$,
\begin{equation}
\label{eqn:suf:cluster}
\E\left[\sum_{C\in U} \sum_{l\in [K_C]} N_{C,n}^{l, suf}\right] \leq (1-\beta)n+\frac{\pi^2}{3}\cdot m
\end{equation}
\end{mylem}
\begin{proof}
By the definition of $N_{C,n}^{l,suf}$, it is sufficient to show that for any $t>m$,
\begin{align*}
&\E\left[ \sum_{C\in [m], l\in [K_C]}\I\{S_t= S_{C,\bad}^l, N_{C,t}>N_{C,t-1}, N_{C,t-1} > \ell_n(\Delta^{C,l})\}\right]\\
\le&\sum_{C\in[m], l\in [K_C]}\Pr\{ S_t = S_{C,\bad}^l, \forall s \in S_{C,\bad}^l, T_{s,t-1} > \ell_n(\Delta^{C,l}) \}
\\ \leq &(1-\beta)+2mt^{-2}\\
\end{align*}
Define $\Lambda_{i,t}=\sqrt{ \frac{
%2\ln t+\ln \ln t
3\ln t}{2T_{i,t-1}}}$ (a random variable
	since $T_{i,t-1}$ is a random variable)
	and $\Lambda_{t}
	%\stackrel{\mathrm{def}}{=}
	=\max \{
	\Lambda_{i,t} \,\mid i\in S_t\}$.
Define $\Lambda^{C,l} = \sqrt{\frac{3\ln t}{2\ell_n(\Delta^{C,l})}}$.

Let $\calN_t$ indicate the event that the process is {\em nice} at time $t$. Let $F_t$ indicate
the event that the oracle fails to return an $\alpha$-approximation with respect to the input vector at time $t$.
For any particular $C\in U$ and $l\in [K_C]$, if  $\left\{\calN_t, \neg F_t, S_t = S_{C,\bad}^l,
\forall s\in S_t, T_{s,t-1} >\base_n(\Delta^{C,l})
\right\}$ holds at time $t$, we have the following properties:
\begin{align*}
r_{\bp}(S_t) + f(2\Lambda^{C,l}) >& r_{\bp}(S_t) +f(2\Lambda_{t})
&\mbox{
  strict monotonicity of $f(\cdot)$ and %  Eq.(\ref{eqn:deltal>deltat})}\\ --YY
  Eq.(8)}\\
\geq &
r_{\bar{\bp}_t}(S_t)  &\mbox{bounded smoothness property and %Eq.(\ref{eqn:op-p<2deltat})} --YY
Eq.(7)}
\\
\geq &\alpha\cdot {\opt_{\bar{\bp}_t}}&
	\mbox{$\neg F_t \Rightarrow$  $S_t$ is an $\alpha$
  approximation w.r.t $\bar{\bp}_t$}
\\
\geq &\alpha \cdot r_{\bar{\bp}_t}(S_\bp^*)
&\mbox{definition of $\opt_{\bar{\bp}_t}$}
\\
\geq & \alpha\cdot r_{\bp}(S_\bp^*)
 = \alpha\cdot \opt_{\bp}. &\mbox{ monotonicity of $r_{\bp}(S)$ and % Eq.(\ref{eqn:op>p})}  --YY
 Eq.(9)}
\end{align*}

So we have
\begin{align}
r_{\bp}(S_{C,\bad}^l)+f(2\Lambda^{C,l})> \alpha \cdot \opt_\bp.
 \label{eqn:min_Delta_il:cluster}
\end{align}

Since  $\base_n(\Delta^{C,l}) = \frac{
6\ln n
 }{(f^{-1}(\Delta^{C,l}))^2}$,
we have
$f(2\Lambda^{C,l}) =\Delta^{C,l}$.
Therefore,
Eq.~(\ref{eqn:min_Delta_il:cluster}) contradicts the definition of
	$\Delta^{C,l}$.
In other words,
\begin{align*}
&\forall C\in[m]\, \forall l\in[K_C],\,
\Pr \left\{\calN_t, \neg F_t, S_t=S_{C,\bad}^l,
\forall s\in S_t, N_{s,t-1} >\base_n(\Delta^{C,l})
\right\}  = 0  \\ \Rightarrow
&\Pr\left\{\calN_t, \neg F_t, \exists C\in U, \exists l\in [K_C],   S_t=S_{C,\bad}^l,
\forall s\in S_t,  N_{s,t-1} >\base_n(\Delta^{C,l})
\right\} = 0   \\ \Rightarrow
&\Pr \left\{\exists C\in U, \exists l\in [K_C],   S_t=S_{C,\bad}^l,
\forall s\in S_t,  N_{s,t-1} >\base_n(\Delta^{C,l})
\right\} \leq \Pr[F_t \lor \neg \calN_t] \leq (1-\beta)+2mt^{-2} \\ \Rightarrow
&\sum_{C\in U,l\in[K_C]}\Pr \left\{ S_t=S_{C,\bad}^l,
\forall s\in S_t, N_{s,t-1} >\base_n(\Delta^{C,l})
\right\} \leq (1-\beta)+2mt^{-2}
\end{align*}

The first inequality comes from Lemma~\ref{lem:nice}.
\end{proof}

Now we consider the bad super arms that are under-sampled when played. To simplify the notation, define $\ell_n(\Delta^{C,0}) = 0$. For a cluster $C$,

\begin{align}
&\sum_{l\in [K_C]} N_{C,n}^{l,und}\cdot \Delta^{C,l} \nonumber\\
=& \sum_{t=|U|+1}^n \sum_{l\in [K_C]}\I\{S_t = S_{C,\bad}^l, N_{C,t}>N_{C,t-1}, N_{C,t-1} \le \ell_n(\Delta^{C,l})\}\cdot \Delta^{C,l} \nonumber\\
=& \sum_{t=|U|+1}^n \sum_{l\in [K_C]} \sum_{j=1}^l \I\{S_t = S_{C,\bad}^l, N_{C,t}>N_{C,t-1}, N_{C,t-1} \in (\ell_n(\Delta^{C,j-1}), \ell_n(\Delta^{C,j}) ] \} \cdot \Delta^{C,l} \nonumber\\
\leq& \sum_{t=|U|+1}^n \sum_{l\in [K_C]} \sum_{j=1}^l \I\{S_t = S_{C,\bad}^l, N_{C,t}>N_{C,t-1}, N_{C,t-1} \in (\ell_n(\Delta^{C,j-1}), \ell_n(\Delta^{C,j}) ] \} \cdot \Delta^{C,\mathbf{j}} \nonumber\\
\leq& \sum_{t=|U|+1}^n \sum_{l\in [K_C]} \sum_{j\in [\mathbf{K_C}]} \I\{S_t = S_{C,\bad}^l, N_{C,t}>N_{C,t-1}, N_{C,t-1} \in (\ell_n(\Delta^{C,j-1}), \ell_n(\Delta^{C,j}) ] \} \cdot \Delta^{C,j} \nonumber\\
%=& \sum_{t=|U|+1}^n \sum_{j\in [K_C]} \sum_{l\in [K_C]} \I\{S_t = S_{C,\bad}^l, N_{C,t}>N_{C,t-1}, N_{C,t-1} \in (\ell_n(\Delta^{C,j-1}), \ell_n(\Delta^{C,j}) ] \} \cdot \Delta^{C,l} \nonumber \\
%\le &\sum_{t=|U|+1}^n \sum_{j\in [K_C]} \sum_{l=j}^{K_C} \I\{S_t = S_{C,\bad}^l, N_{C,t}>N_{C,t-1}, N_{C,t-1} \in (\ell_n(\Delta^{C,j-1}), \ell_n(\Delta^{C,j}) ] \} \cdot \Delta^{C,j} \nonumber \\
=& \sum_{t=|U|+1}^n \sum_{j\in [K_C]} \I\{S_t \in \calS_{C,\bad}, N_{C,t}>N_{C,t-1}, N_{C,t-1} \in (\ell_n(\Delta^{C,j-1}), \ell_n(\Delta^{C,j}) ] \} \cdot \Delta^{C,j} \nonumber \\
=&  \sum_{j\in [K_C]} \sum_{t=|U|+1}^n\I\{S_t \in \calS_{C,\bad}, N_{C,t}>N_{C,t-1},  N_{C,t-1} \in (\ell_n(\Delta^{C,j-1}), \ell_n(\Delta^{C,j}) ] \} \cdot \Delta^{C,j} \nonumber \\
\leq& \sum_{j\in [K_C]} (\ell_n(\Delta^{C,j}) - \ell_n(\Delta^{C,j-1}))\cdot \Delta^{C,j} \nonumber\\
=& \ell_n(\Delta^{C,K_i}) \Delta^{C,K_i}+\sum_{j\in [K_C]} \ell_n(\Delta^{C,j}) \cdot( \Delta^{C,j} -\Delta^{C,j+1})
\nonumber \\
\leq& \ell_n(\Delta^{C,K_C}) \Delta^{C,K_C} + \int_{\Delta^{C,K_C}}^{\Delta^{C,1}} \ell_n(x) \mathrm{d}x.
\label{eqn:und:cluster}
\end{align}

Last inequality comes from the fact that $\ell_n(x)$ is decreasing.
Notice that by our definition, for clusters that $C_j \in [m] \setminus \{ C \mid \Delta_{\min}^C > 0 \}$, the counter $N_C$ remains one after the initialization. Since they do not contribute to any regret, we have $K_C = 0$ for all these arms.
Combining with Eq.(\ref{eqn:suf:cluster}) and Eq.(\ref{eqn:und:cluster}), the overall regret of our algorithm is
\begin{align*}
& Reg^A_{\bp,\alpha,\beta}(n)
\\ \leq &n \cdot \alpha  \cdot
\beta\cdot  \opt_{\bp}  -
\left(\alpha \cdot n\cdot \opt_{\bp} -  \sum_{C\in U}\left( \Delta^{C,1}+\sum_{l\in [K_C]} (N_{C,n}^{l, suf} + N_{C,n}^{l, und}) \cdot \Delta^{C,l}\right) \right)\\
\leq& \Delta_{\max} \cdot \sum_{C\in U, l\in [K_C]} N_{C,n}^{l, suf}
+ \sum_{C\,\mid \, \Delta_{\min}^C > 0}\left( \Delta^{C,1}+ \ell_n(\Delta^{C,K_C}) \Delta^{C,K_C} +  \int_{\Delta^{C,K_C}}^{\Delta^{C,1}} \ell_n(x) \mathrm{d}x\right) - (1-\beta)\cdot n\cdot \alpha \cdot \opt_{\bp}\\
\leq &\left(\frac{\pi^2}{3}+1\right)\cdot m \cdot \Delta_{\max} +
\sum_{C\,\mid \, \Delta_{\min}^C > 0}\left( \ell_n(\Delta^{C,K_C}) \Delta^{C,K_C} + \int_{\Delta^{C,K_C}}^{\Delta^{C,1}} \ell_n(x) \mathrm{d}x\right) .
\end{align*}
The theorem follows directly.
\end{proof}

\vspace{\subsectionspace}
\section{$\varepsilon_t$-Greedy algorithm}
\vspace{\subsectionspace}

\begin{algorithm}[t]
    \centering
    \caption{$\varepsilon_t$-greedy algorithm with computation oracle}
    \label{alg:epsgreedy}
    \begin{algorithmic}[1]
        \STATE For each arm $i$, maintain variable $\hat \mu_{i}$ as the
	mean of all outcomes $X_{i,*}$'s of arm $i$ observed so far.
        \STATE $\myn\leftarrow 0$
        \WHILE {\TRUE}
            \STATE $\myt\leftarrow \myt+1$; $\varepsilon_\myt\leftarrow\min\{\frac{\gamma}{\myt},1\}$.
            \STATE With probability $\varepsilon_\myt$, choose an arm $i$
            uniform at random, then play an arbitrary super arm $S\in\calS$ containing
            $i$; with probability $1-\varepsilon_\myt$,
            get $S = \mathrm{Oracle}(\hat \mu_1,
            \hat \mu_2,\ldots, \hat \mu_m)$.
            \STATE Play $S$ and update all $\hat \mu_{\myi}$'s.
        \ENDWHILE
    \end{algorithmic}
\end{algorithm}
Unlike CUCB algorithm,
$\varepsilon_t$-greedy algorithm
exhibits the combination of exploration and exploitation more explicitly.
In the $\myt$-th round,
with probability $\varepsilon_\myt$
the algorithm  performs {\em exploration},
i.e.,  chooses an  arm  $i$ uniformly at random, then select an arbitrary
super arm $S\in \calS$ containing $i$;
with probability $1-\varepsilon_\myt$,
the algorithm  performs {\em exploitation},
i.e., uses the approximation oracle to choose a super arm.
As $\myt$ grows,
the probability of performing
exploration decreases so that the regret can be bounded. See
Algorithm \ref{alg:epsgreedy} for details.
Note that if an arm $i$ has never been played, $\hat \mu_i$ could be any
	arbitrary value.

The appeal of the $\epsilon_t$-greedy algorithm is its simplicity and
	match with intuition.
However, as shown in the following theorem, in order to have a theoretical
	guarantee on the regret bound, parameter $\gamma$ needs to be set
	appropriately and it depends on $\Delta_{\min}$ and function $f(\cdot)$.
In constrast, the CUCB algorithm does not rely on the knowledge of
	$\Delta_{\min}$ and $f(\cdot)$, and thus CUCB is applicable to more
	settings in this sense.

\begin{mythm} \label{thm:epsgreedy}
{\thmepsgreedy}
\end{mythm}

Recall that the definition of $\Delta_{\min}$ is
\begin{equation}
\label{eqn:gmin}
\Delta_{\min} = \alpha\cdot \opt_{\bp} - \max\{ r_{\bp}(S) \, \mid \, S\in \calS_\bad\}.
\end{equation}

\begin{proof}
Let $R_{\myi,\myt}$ be the indicator for the event that $\myi$ was
chosen to {\em explore} in  the $\myt$-th round and $N_{i,t}$ be the
number of rounds that arm $i$ is explored in the first $t$ rounds.
Set $\varphi = \frac{\gamma}{3m}$.
For simplicity, we assume $\gamma$ is integer.
We have:
\begin{align}
%\mathbb{E}[\myn^\myR_{\myi,\myn}]=
\E[N_{i,n}] = \sum_{\myt=1}^\myn \mathbb{E}[R_{\myi,\myt}]=
\sum_{\myt=1}^\myn \frac{\varepsilon_\myt}{m}=
\frac{\gamma-1}{m}+
\sum_{\myt=\gamma}^\myn \frac{3\varphi}{\myt}
>  3\varphi+ \int_{\gamma}^{\myn} \frac{3\varphi}{\myx} \dx=
1+ 3\varphi \ln (\myn /\gamma)
\label{ineq1}
\end{align}
When $n> \gamma ^3$,  (\ref{ineq1}) is at least $2\varphi \ln n  +
1$. Now let
$\myX_{\myi,\myt}=R_{\myi,\myt}-\mathbb{E}[R_{\myi,\myt}]$. We
have $\mathbb{E}[\myX_{\myi,\myt}]=0$,
 $|\myX_{\myi,\myt}|\leq 1$, and
\begin{align*}
\sum_{\myt=1}^\myn\mathbb{E} \left[\myX_{\myi,\myt}^2\right]=
% Yajun: for t<gamma, X is equal to 0
%\sum_{\myt=1}^{\gamma-1}
%\left(1-\frac{1}{m}\right)\frac{1}{m}+
\sum_{\myt= \gamma }^\myn\left(1-\frac{3\varphi}{\myt}\right)\frac{3\varphi}{\myt}<
3\varphi \ln \myn.
\end{align*}
By Bernstein inequality in Lemma \ref{bernstein}, when $n>
\gamma^3$, we have
\begin{align*}
\Pr \left[\left|\sum_{\myt=1}^\myn \myX_{\myi,\myt}\right|>\varphi \ln
  \myn \right] &\leq \exp\left\{-\frac{\varphi^2(\ln \myn)^2 /2}
{\sum_{\myt=1}^\myn \mathbb{E} [\myX_{\myi,\myt}^2]+\myM (\varphi \ln  \myn)/3}\right\}\nonumber\\
&\leq \exp\left\{-\frac{\varphi^2(\ln \myn)^2 /2}
{3\varphi \ln \myn+\varphi \ln  \myn/3}\right\}\nonumber\\
&=\mye^{-\frac{3}{20}\varphi\ln \myn}=\myn^{-\frac{3}{20}\varphi}\leq n^{-c}.
\end{align*}
In other words, $\Pr[ N_{i,t} \leq \varphi \ln t +1] \leq
t^{-c}$. By union bound, $\Pr[\exists i\in [m], \, N_{i,t} \leq
\varphi \ln t  +  1] \leq mt^{-c}$.
Let $P_t$ to be the indicator of the event that in the $t$-th round, all
the arms have been played for at least $\varphi \ln t  +1$
times.
So, $\Pr[P_t=0]\leq mt^{-c}$.
Set $\base_t=
\frac{(c+1) \ln t}
{\left(f^{-1}
\left(\frac{\Delta_{\min}}{2}\right)\right)^{2}}
\leq \varphi \ln t
$.
Note $P_t=1$ indicates for every arm $i$,
$T_{i,t}\geq N_{i,t}\geq \varphi \ln t  +1>\base_t$.

Let $I_{t}$ be the event that
we choose a bad arm $S_t\in \calS_{\bad}$ in the
$t$-th round. Let $Y_{t}$
be the event that
the action taken in the $t$-th round
is exploitation (not exploration).
Let $F_t$ be the event that the oracle failed to produce an
$\alpha$-approximate answer in an exploitation round $t$.
We have $\mathbb{E}[F_t\mid Y_{t}]\leq 1-\beta$.

We have,
\begin{align*}
\sum_{t=\gamma^3+1}^n  \I \{I_t\}
&=
\sum_{t=\gamma^3+1}^n
\left(\I\{I_t,\neg Y_t\}+\I\{I_t,Y_t\}\right)
\\
&=
\sum_{t=\gamma^3+1}^n
\varepsilon_t\cdot \I\{I_t \mid \neg Y_t\}+
\sum_{t=\gamma^3+1}^n
\I\{I_t, Y_t\}
\\
&\leq
\gamma \ln n+
\sum_{t=\gamma^3+1}^n
\I\{I_t ,Y_t\}
\end{align*}

Consider the second term.
\begin{align*}
\\
&\sum_{t=\gamma^3+1}^n
\I\{I_t, Y_t\}
\\
\leq &
\sum_{t=\gamma^3+1}^n
\left(\I\{F_t, Y_t\}
+\I\{\neg F_t, I_t, Y_t\}
\right)
\\\leq&
(1-\beta)(n-\gamma^3)+
\sum_{t=\gamma^3+1}^n
\left(
\I\{\neg F_t,I_t,\neg P_t , Y_t\}
+\I\{\neg F_t,I_t,P_t, Y_t\}
\right)
\\
\leq&
(1-\beta)n+
\sum_{t=\gamma^3+1}^n
\left(
mt^{-c}\cdot \I\{I_t\mid \neg F_t,\neg P_t,Y_t\}
+\I\{\neg F_t,I_t, P_t, Y_t\}
\right)
\\
\leq&
(1-\beta)n+
\zeta(c)\cdot m+
\sum_{t=\gamma^3+1}^n
\I\{\neg F_t,I_t,P_t,  Y_t\}
\\
=&
(1-\beta)n+
\zeta(c)\cdot m+
\sum_{t=\gamma^3+1}^n
%\sum_{S^j\in \calS_\bad}
%\sum_{i\in S^j \atop \base_t< s_i<t}
\I\{
\neg F_t,Y_t, S_t\in \calS_\bad,
\forall i\in [m],\, T_{i,t-1}>\base_t
\}\nonumber
\end{align*}

We claim that
$$\Pr[\{
\neg F_t,Y_t, S_t\in \calS_\bad,
\forall i\in [m],\, T_{i,t-1}>\base_t
\}] \leq 2\cdot m\cdot t^{-c}.
$$
We now prove this claim.
%Same as in the proof of Theorem~\ref{thm:cucb individual}, --YY
Same as in the proof of Theorem~1,
	let $T_{i,n}$ be the number of times arm $i$ is played in the
	first $n$ rounds;
	let $\hat \mu_{i,s}$ be the value of $\hat \mu_i$ after
	arm $i$ is played $s$ times, that is,
	$\hat \mu_{i,s} = (\sum_{j=1}^{s} X_{i,j})/s$.
Then, the value of variable $\hat \mu_i$ at the end of round $n$
	is $\hat \mu_{i,T_{i,n}}$.
By Chernoff bound in Lemma~\ref{chernoffLemma},
for any $i\in [m]$,
\begin{align}
\Pr\left[
|\hat \mu_{i,T_{i,t-1}} - \mu_i|
\geq  \sqrt{\frac{
2\ln t+\ln \ln t
}{2T_{i,t-1}}}
\right]
%& = \sum_{s=1}^{t-1} \Pr\left[
%\left\{ |\hat p_{i,s} - p_i|
%\geq  \sqrt{\frac{
%(c+1)\ln t
%}{2s} }, T_{i,t-1} = s
%\right\}
%\right] \nonumber\\
%& \leq \sum_{s=1}^{t-1} \Pr\left[
%\left\{ |\hat p_{i,s} - p_i|
%\geq  \sqrt{\frac{
%(c+1)\ln t
%}{2s} }
%\right\}
%\right] \nonumber\\
&\leq t\cdot 2e^{-2\ln t - \ln \ln t}
\leq 2(t\ln t)^{-1}. \label{eqn:epsilonhatp-p}
\end{align}

Define $\Delta_{i,t}=\sqrt{ \frac{2\ln t + \ln\ln t}{2T_{i,t-1}}}$.
Define $\cF_t = \{ \forall i \in [m], \,
|\hat \mu_{i,T_{i,t-1}} -  \mu_i|  \leq \Delta_{i,t}\}$.
By union bound, $\Pr[\neg \cF_t] \leq 2\cdot m \cdot t^{-c}$.
Let $\Delta = \sqrt{\frac{2\ln t+\ln\ln t}{2\base_t}}$. Notice that when $\forall i\in [m], T_{i,t-1}>\base_t$, we have $\Delta
> \Delta^t \stackrel{\mathrm{def}}{=} \max \{ \Delta_{i,t} \,\mid i\in [m]\}$.

Let $\hat{\bp}_t = (\hat{\mu}_{1,T_{1,t-1}}, \ldots, \hat{\mu}_{m,T_{m,t-1}})$ be
	the random vector representing the
	estimated expectation vector at round $t$ before calling the oracle.
	Then,
when $\{\cF_t, \neg F_t, Y_t, S_t\in \calS_\bad, \forall i\in [m], T_{i,t-1}>\base_t\}$ holds, we have the following properties:
\begin{align*}
r_{\bp}(S_t)+2f(\Delta) & >
r_{\bp}(S_t)+(1+\alpha)f(\Delta^t) &\mbox{monotonicity of $f(\cdot)$}\\
&\geq r_{\hat\bp_t}(S_t)+\alpha f(\Delta^t)
& \mbox{bounded smoothness property with $\cF_t$}\\
&\geq \alpha\cdot \opt_{\hat \bp_t}+\alpha f(\Delta^t)
& \mbox{$\neg F_t \Rightarrow$  $S_t$ is an $\alpha$
  approximation w.r.t $\hat{\bp}_t$}\\
& \geq \left(r_{\hat\bp_t}(S_\bp^*)+f(\Delta^t)\right)\cdot \alpha
&\mbox{definition of $\opt_{\hat{\bp}_t}$} \\
&\geq \alpha \cdot r_{\bp}(S_\bp^*) = \alpha \cdot \opt_{\bp}. &
\mbox{bounded smoothness property with $\cF_t$}
\end{align*}

These above inequalities imply that when $\cF_t$ holds,  we have
\begin{align}
r_\bp(S^j) +2f(\Delta) > \alpha \cdot \opt_\bp.
\label{eqn:sopt}
\end{align}

Since  $\base_t = \frac{
2\ln t+\ln\ln t
 }{\left(f^{-1}\left(\frac{\Delta_{\min}}{2}\right)\right)^2}$,
we have
\[
2f(\Delta)
=2f\left(f^{-1}\left(\frac{\Delta_{\min}}{2}\right)\right)
=\Delta_{\min}.
\]
With $2f(\Delta)=\Delta_{\min}$, Eq.~(\ref{eqn:sopt}) is in conflict
	with the definition of $\Delta_{\min}$ in Eq.~(\ref{eqn:gmin}).
In other words,
\begin{align*}
&\Pr\left[ \{
\cF_t, \neg F_t,Y_t, S_t\in \calS_\bad,
\forall i\in [m], T_{i,t-1}>\base_t
\}\right] = 0 \Rightarrow \\
&\Pr\left[ \{\neg F_t,Y_t, S_t=S^j,
\forall i\in S^j \cup S_\bp^*, T_{i,t-1}=s_i
\} \right] \leq \Pr[\neg \cF_t]\leq
2\cdot m\cdot (t\ln t)^{-1}.
\end{align*}

Thus,
\begin{align*}
&\E\left[\sum_{t=1}^n \I \{I_t\}\right]
\\
\leq &
\gamma^3+
\gamma \ln n +
(1-\beta)n+
\zeta(c)\cdot m+
\sum_{t=\gamma^3+1}^n 2\cdot m (t\ln t)^{-1}
\\
\leq &
\gamma^3+\gamma \ln n +(1-\beta)n+
\zeta(c)\cdot m + 2m\ln \ln n
\end{align*}

That means, the regret is at most:
\begin{align*}
Reg^A_{\bp,\alpha,\beta}(n) &\leq n \cdot \alpha  \cdot
\beta\cdot  \opt_{\bp}  -
\left( n\cdot \alpha\cdot
  \opt_{\bp}-\Delta_{\max}\cdot
  \mathbb{E}\left[\sum_{t=1}^n \I \{I_t\}\right]\right)
  \\&\leq
\left(
\gamma^3+\gamma \ln n +(1-\beta)n+
3\cdot \zeta(c)\cdot m
\right)\Delta_{\max} -
(1-\beta) \cdot n \cdot \alpha \cdot \opt_{\bp} \nonumber\\
&\leq
\left(
\gamma \ln n +
3\cdot \zeta(c)\cdot m
+ \gamma ^3
\right) \Delta_{\max}.
\end{align*}

\end{proof}

\section{Improving the UCB1 algorithm of~\cite{AuerCF02} and its analysis
	using our approach} \label{sec:improveUCB1}

We can improve the UCB1 algorithm of~\cite{AuerCF02} by replacing
	its adjustment term of $\sqrt{\frac{2\ln n}{n_i}}$
	with $\sqrt{\frac{(c+1)\ln n}{2n_i}}$ for any $c>1$.
The improved analysis using our approach will give the following regret
	bound:
\[
\left[ 2(c+1) \sum_{i:\mu_i < \mu^*} \left( \frac{\ln n}{\Delta_i}\right)\right]
	+ \left(1+2\cdot \zeta(c)\right)\left(\sum_{j=1}^{K} \Delta_j\right).
\]

The following is the revised analysis of the improved algorithm.
We start from the following formula in page 242 of the paper~\cite{AuerCF02}:
\begin{align*}
T_i(n) \le \ell + \sum_{t=K+1}^n\I\{\bar{X}^*_{T^*(t-1)} + c_{t-1,T^*(t-1)}
	 \le \bar{X}_{i,T_i(t-1)} + c_{t-1,T_i(t-1)}, T_i(t-1)\ge \ell\}.
\end{align*}
Following the argument of the paper, event
	$\{\bar{X}^*_{T^*(t-1)} + c_{t-1,T^*(t-1)}
	\le \bar{X}_{i,T_i(t-1)} + c_{t-1,T_i(t-1)}\}$ implies that
	$\{\bar{X}^*_{T^*(t-1)} \le \mu^*- c_{t-1,T^*(t-1)}\}$ or
	$\{\bar{X}_{i,T_i(t-1)}  \ge \mu_i + c_{t-1,T_i(t-1)}\}$ or
	$\{\mu^* < \mu_i + 2c_{t-1,T_i(t-1)}\}$.
Therefore, we have
\begin{align}
&T_i(n)\nonumber\\
\le& \ell + \sum_{t=K+1}^n\I\{\bar{X}^*_{T^*(t-1)} + c_{t-1,T^*(t-1)}
\le \bar{X}_{i,T_i(t-1)} + c_{t-1,T_i(t-1)}, T_i(t-1)\ge \ell \} \nonumber\\
   \le&  \ell
   	+\sum_{t=K+1}^n [
\I\{\mu^* < \mu_i + 2c_{t-1,T_i(t-1)}, T_i(t-1)\ge \ell\}
   +
	\I\{\bar{X}^*_{T^*(t-1)} \le \mu^*- c_{t-1,T^*(t-1)}, T_i(t-1)\ge \ell\}
\nonumber\\
	&
+\I\{\bar{X}_{i,T_i(t-1)}  \ge \mu_i + c_{t-1,T_i(t-1)}, T_i(t-1)\ge \ell\}
	] \label{eq:key}\\
 \le&  \ell + \sum_{t=K+1}^n
	\I\{\bar{X}^*_{T^*(t-1)} \le \mu^*- c_{t-1,T^*(t-1)}\} +
	\sum_{t=K+1}^n\I\{\bar{X}_{i,T_i(t-1)}  \ge \mu_i + c_{t-1,T_i(t-1)}\}
\nonumber\\ & +
	\sum_{t=K+1}^n\I\{\mu^* < \mu_i + 2c_{t-1,T_i(t-1)}, T_i(t-1)\ge \ell\} \nonumber\\
 \le & \ell + \sum_{t=K+1}^n\sum_{s=1}^{t-1}
	\I\{\bar{X}^*_{s} \le \mu^*- c_{t-1,s}\} +
	\sum_{t=K+1}^n\sum_{s_i=1}^{t-1}
	\I\{\bar{X}_{i,s_i}  \ge \mu_i + c_{t-1,s_i}\} \nonumber\\&+
	\sum_{t=K+1}^n \I\{\mu^* < \mu_i + 2c_{t,T_i(t-1)}, T_i(t-1)\ge \ell\} \nonumber\\
 \le & \ell + \sum_{t=1}^\infty\sum_{s=1}^{t}
	\I\{\bar{X}^*_{s} \le \mu^*- c_{t,s}\} +
	\sum_{t=1}^\infty\sum_{s_i=1}^{t}
	\I\{\bar{X}_{i,s_i}  \ge \mu_i + c_{t,s_i}\} +
	\sum_{t=K+1}^n \I\{\mu^* < \mu_i + 2c_{t,T_i(t-1)}, T_i(t-1)\ge \ell\}. \nonumber
\end{align}

Derivation on Eq.~\eqref{eq:key} is the key.
It uses fixed values $\mu^*$ and $\mu$ to separate two sets of
	 random variables and their inequalities.
The enumeration of the values of those random variables only comes after,
	where the original proof does the enumeration first,which
	has to be $t^2$ combinations.

We set $c_{t,s}=\sqrt{\frac{(c+1)\ln t}{2s}}$, here $c>1$.
This means the UCB algorithm should use adjustment term
	of $\sqrt{\frac{(c+1)\ln n}{2n_i}}$.
Then by Chernoff bound, we have
\begin{align*}
\Pr[\bar{X}^*_{s} \le \mu^*- c_{t,s}] \le t^{-(c+1)} ,~~
\Pr[\bar{X}_{i,s_i}  \ge \mu_i + c_{t,s_i}] \le t^{-(c+1)}.
\end{align*}

Set $\ell = \lceil (2(c+1)\ln n)/\Delta_i^2 \rceil$.
Then when $t\le n$ and $T_i(t-1) \ge \ell$,
	$2c_{t,T_i(t-1)} \le 2 c_{t,\ell} \le \Delta_i=\mu^* - \mu_i$.
Therefore, when $t\le n$, indicator
	$\I\{\mu^* < \mu_i + 2c_{t,T_i(t-1)}, T_i(t-1)\ge
	\lceil (2(c+1)\ln n)/\Delta_i^2 \rceil\}$ is always $0$.
Hence, we have

\begin{align*}
&\mathbb{E}[T_i(n)] \\ \le& \left\lceil \frac{2(c+1)\ln n}{\Delta_i^2}\right\rceil +
	\sum_{t=1}^\infty\sum_{s=1}^{t}
	\Pr[\bar{X}^*_{s} \le \mu^*- c_{t,s}] +
	\sum_{t=1}^\infty\sum_{s_i=1}^{t}
	\Pr[\bar{X}_{i,s_i}  \ge \mu_i + c_{t,s_i}] +\\&
	\sum_{t=K+1}^n \Pr\left[\mu^* < \mu_i + 2c_{t,T_i(t-1)}, T_i(t-1)\ge
	\left\lceil \frac{2(c+1)\ln n}{\Delta_i^2}\right\rceil\right] \\
	 \le &\left\lceil \frac{2(c+1)\ln n}{\Delta_i^2}\right\rceil +
	2\sum_{t=1}^\infty\sum_{s=1}^{t} t^{-(c+1)}
	\le \frac{2(c+1)\ln n}{\Delta_i^2} + 1 + 2\cdot \zeta(c).
\end{align*}
Therefore, the regret bound is given by
\begin{align*}
&\sum_{i:\mu_i < \mu^*} \mathbb{E}[T_i(n)]\cdot\Delta_i \le
\left[ 2(c+1) \sum_{i:\mu_i < \mu^*} \left( \frac{\ln n}{\Delta_i}\right)\right]
	+ \left(1+2\cdot \zeta(c)\right)\left(\sum_{j=1}^{K} \Delta_j\right),
\end{align*}
with any $c>1$.

The analysis in~\cite{AuerCF02} corresponds to the special case of $c=2$,
	for which we have the following bound.
\begin{align*}
&\sum_{i:\mu_i < \mu^*} \mathbb{E}[T_i(n)]\cdot\Delta_i \le
\left[ 6 \sum_{i:\mu_i < \mu^*} \left( \frac{\ln n}{\Delta_i}\right)\right]
	+ \left(1+\frac{\pi^2}{3}\right)\left(\sum_{j=1}^{K} \Delta_j\right).
\end{align*}
The constant coefficient of the leading term is reduced from $8$ to $6$.
We can further choose any $c>1$ and reduce the coefficient to
	$2(c+1)$, making it arbitrarily close to $4$.
